# Supplementary material for: One-Shot Imitation Learning with Invariance Matching for Robotic Manipulation
Source: arXiv:2405.13178 source file (2024-06-05)
Supplement: Supplementary file 1 [file 8.appendix.tex]

\section{Implementation Details}
\label{apn:impl}
